# Supplementary material for: Provably Efficient Reinforcement Learning for Online Adaptive Influence Maximization
Source: arXiv:2206.14846 source file (2022-06-29)
Supplement: Supplementary file 1 [file appendix.tex]

\section{Appendix}

Optionally include extra information (complete proofs, additional experiments and plots) in the appendix.
This section will often be part of the supplemental material.
